# Supplementary material for: LineGS : 3D Line Segment Representation on 3D Gaussian Splatting
Source: arXiv:2412.00477 source file (2024-12-13)
Supplement: Supplementary file 1 [file Appendix.tex]

\section*{}
